# Supplementary material for: Statistical Reachability Analysis of Stochastic Cyber-Physical Systems under Distribution Shift
Source: arXiv:2407.11609 source file (2024-07-16)
Supplement: Supplementary file 1 [file appendix.tex]

\subsection{Training the Scaling Factors with Surrogate Model}\label{apdx:scalor}

 Our ultimate goal for training a surrogate model is to receive the smallest flowpipe that covers the trajectories of the underlying system with a provable guarantee. Therefore, in this study, we add a regularization to  the mean square error $\mathbf{MSE}$ loss function to train the parameters of the surrogate model. In another word, we are interested to a small flowpipe, even if it requires a higher level of error for trajectory prediction. In addition, unlike the work, \cite{cleaveland2023conformal} that optimizes the scaling factors $\alpha_i , i\in [n\horizon]$ to minimize the quantile within a LCP optimization framework, here we train these scaling factors to receive the tightest possible flowpipe. Therefore, we propose our Loss function as follows.
 \begin{equation}\label{eq:lossdefinition}
 \mathbf{Loss} = \mathbf{MSE}+\frac{1}{L_2} \sum_{i=1}^{L_2} \max \left[ \left\{\alpha_j R_i^j\right\}_{j=1}^{n\horizon} \right] \left[ \frac{1}{\alpha_1}+\frac{1}{\alpha_2}+\cdots +\frac{1}{\alpha_{n\horizon}} \right],\qquad  R_i^j =  \left|e_{j+n}^\top \traj_{\statee_{0,i}} - \mathsf{F}^j(\statee_{0,i})\right|, \quad  i\in[L_2]
 \end{equation}
 The surface area of the inflating hypercube is given by the formulation:

\[
S = R^* \left( \frac{1}{\alpha_1} + \frac{1}{\alpha_2} + \cdots + \frac{1}{\alpha_{n\horizon}} \right).
\]
Here, \(R^*\) represents the conformalized \(\delta\) quantile of residuals \(R_i = \max \left[ \left\{ \alpha_j R_i^j \right\}_{j=1}^{n\horizon} \right]\), where \(i \in [L]\) from the calibration dataset. It's important to note that the calibration dataset cannot be utilized in the training algorithm. Therefore, there is a need to approximate \(R^*\) with the training dataset, i.e. \(i \in [L_2]\). Approximating \(R^*\) during the training process with the training dataset introduces additional computational complexity, including addressing Karush-Kuhn-Tucker (KKT) conditions (refer to \cite{cleaveland2023conformal}). To simplify, we propose using the expectation of residuals \(R_i, i \in [L_2]\) for training the model instead of their \(\delta\) quantile. This approach is reflected in the loss function defined in \eqref{eq:lossdefinition}. In this training algorithm we use a sampled initial state from training dataset for forward pass to compute the trajectory and then we compute all the component-wise residuals $R^j , j \in [n \horizon]$. We then generate the loss function and use it for backward over both surrogate model parameters and scaling factors. 

% The surface area of the inflating hypercube can be formulated as: 
%  \[
%    S = R^* \left[ \frac{1}{\alpha_1}+\frac{1}{\alpha_2}+\cdots +\frac{1}{\alpha_{n\horizon}} \right]
%  \]
% where $R^*$ is the conformalized $\delta$ quantile of residuals $R_i=\max \left[ \left\{\alpha_j R_i^j\right\}_{j=1}^{n\horizon} \right], i\in [L] $ from the calibration dataset. However, we can not utilize the calibration dataset in the training algorithm, thus we need to approximate $R^*$ with training dataset i.e. $i \in [L_2]$. Approximating $R^*$ in the training process with training dataset also requires more computational complexity (including KKT conditions see \cite{cleaveland2023conformal}) and thus we plan to utilize the expectation residuals $R_i, i\in[L_2]$ for training the model instead of their $\delta$ quantile which results to the loss function proposed in \eqref{eq:lossdefinition}.  
